# Supplementary material for: Real-time 3D-aware Portrait Video Relighting
Source: arXiv:2410.18355 source file (2024-10-24)
Supplement: Supplementary file 1 [file X.Supp.tex]

\setcounter{section}{0}
\setcounter{figure}{0} %

\makeatletter
\def\@maketitle{
   \newpage
   \null
   \begin{center}
      \iftoggle{cvprrebuttal}{{\large \bf \@title \par}}{{\Large \bf \@title \par}}
      \vspace{0.5em}
      \Large{Supplementary Material}
      \vspace{1em}\\
      {
        \large
        \lineskip .5em
        \begin{tabular}[t]{c}
          \iftoggle{cvprfinal}{
            \@author
          }{
            \iftoggle{cvprrebuttal}{}{
              Anonymous \confName~submission\\
              \vspace*{1pt}\\
              Paper ID \paperID
            }
          }
        \end{tabular}
        \par
      }
      \vskip .5em
   \end{center}
}

\makeatother

\maketitle

\section{Additional Results}

\subsection{Additional Qualitative Results}
\Fref{fig:additional novel view relighting} provides
additional qualitative results generated by our relighting technique from portrait videos. %
We encourage readers to refer to the supplementary video for a more comprehensive visualization of our method.

\subsection{Additional Comparisons}

\begin{figure}[htbp] 
\def\lw{0.2857\linewidth}
\def\hlw{0.14285\linewidth}

\centering \small
\begin{tabular}{cccc} 
\includegraphics[width=\lw]{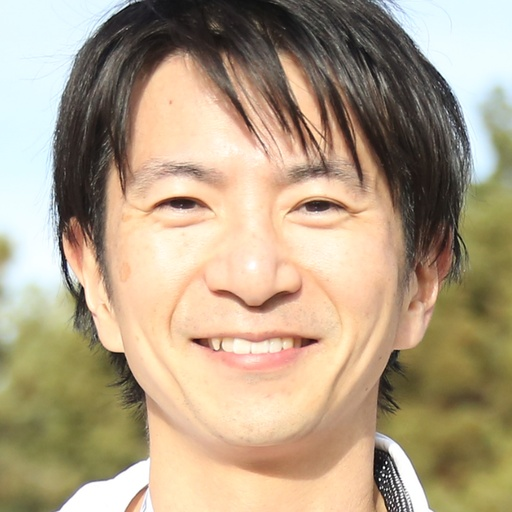} & 
\includegraphics[width=\hlw]{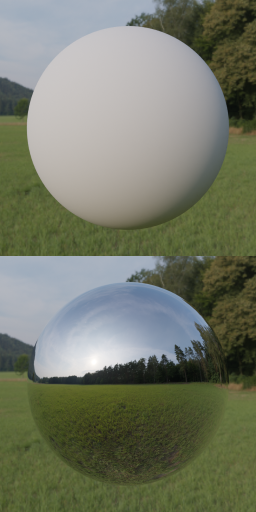} & 
\includegraphics[width=\lw]{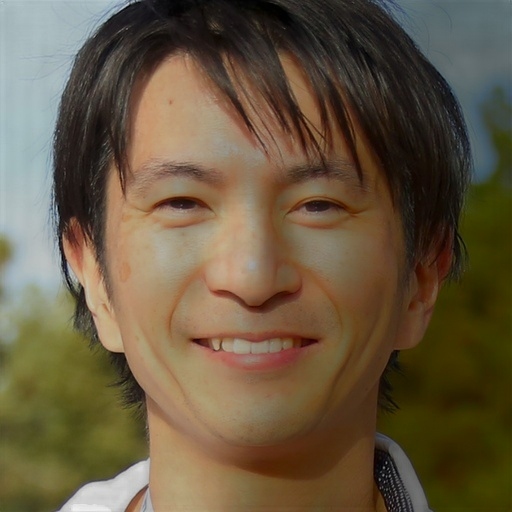}\put(-54,3){\transparent{0.9}\colorbox{gray}{{\textcolor{white}{\footnotesize{\textbf{ID=0.4136}}}}}} & 
\includegraphics[width=\lw]{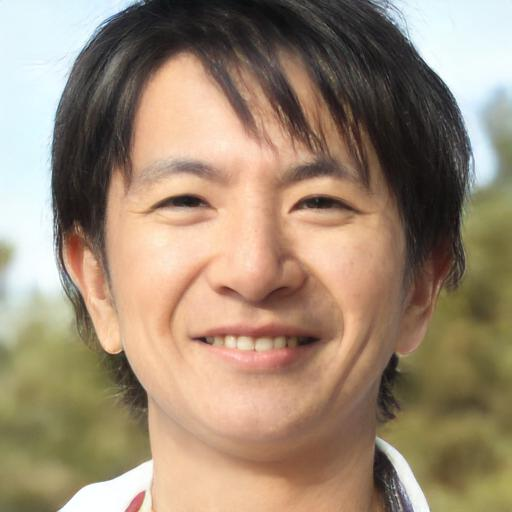}\put(-54,3){\transparent{0.9}\colorbox{gray}{{\textcolor{white}{\footnotesize{\textbf{ID=0.3861}}}}}} \\

\includegraphics[width=\lw]{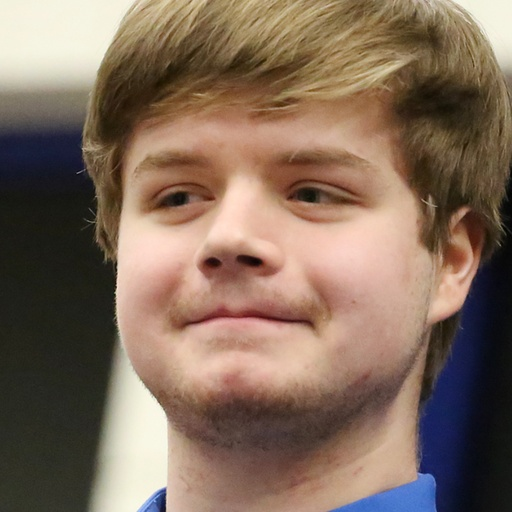} & 
\includegraphics[width=\hlw]{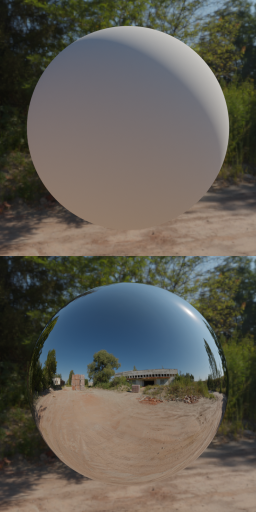} & 
\includegraphics[width=\lw]{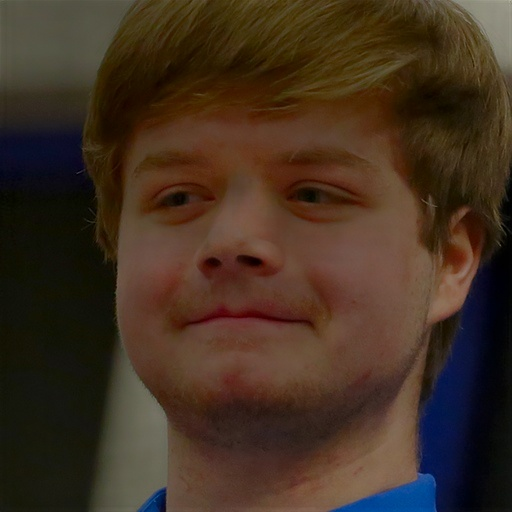}\put(-54,3){\transparent{0.9}\colorbox{gray}{{\textcolor{white}{\footnotesize{\textbf{ID=0.4736}}}}}} & 
\includegraphics[width=\lw]{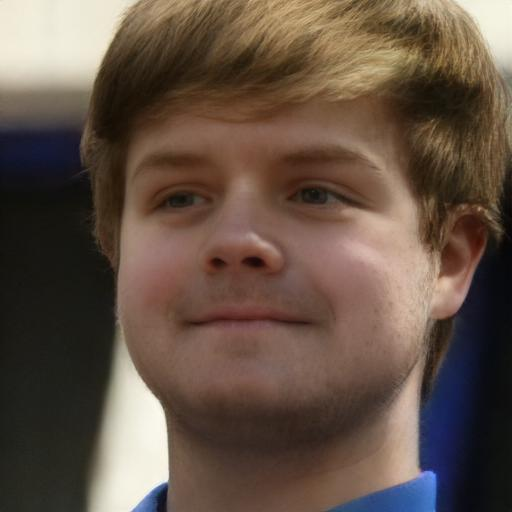}\put(-54,3){\transparent{0.9}\colorbox{gray}{{\textcolor{white}{\footnotesize{\textbf{ID=0.3810}}}}}}  \\
\vspace{0.3mm}
\\
  Input & Light & DPR & Ours
\end{tabular}
\caption{Additional qualitative comparison between %
DPR and ours. Our method consistently delivers portraits with more faithful adherence to desired lighting conditions and enhanced realism.}
\label{fig:additional DPR}
\end{figure}

We conduct a quantitative evaluation for both DPR~\cite{DPR} and our method. It should be noted that %
DPR demonstrates a considerably lower Fréchet Inception Distance (FID) and a higher Identity Perseverance (ID). 
Specifically, the FID is $14.98$ for DPR and $45.08$ for our method, whereas the ID is $0.8531$ for DPR and $0.7711$ for our method. However, these metrics alone do not unequivocally indicate that DPR generates more realistic results, as evidenced in \Fref{fig:additional DPR}. 
The observed differences in FID and ID metrics can be attributed to DPR's underlying approach, which %
operates on the LAB color format. Specifically, DPR selectively modifies only the L channel while keeping the A and B channels unchanged. This strategy results in pixel-wise aligned outputs that closely match the original input. This pixel-wise alignment may contribute to the lower FID and higher ID. 
{However, this approach may lead to a loss of color diversity and realism. Additionally, fine-grained details, particularly color-dependent features, may be inadequately captured, as it neglects changes in the A and B channels.}

\begin{figure*}[htbp] 
\def\lw{1\linewidth}
\def\hlw{0.5\linewidth}

\centering \small
\begin{tabular}{c} 
\includegraphics[width=\lw]{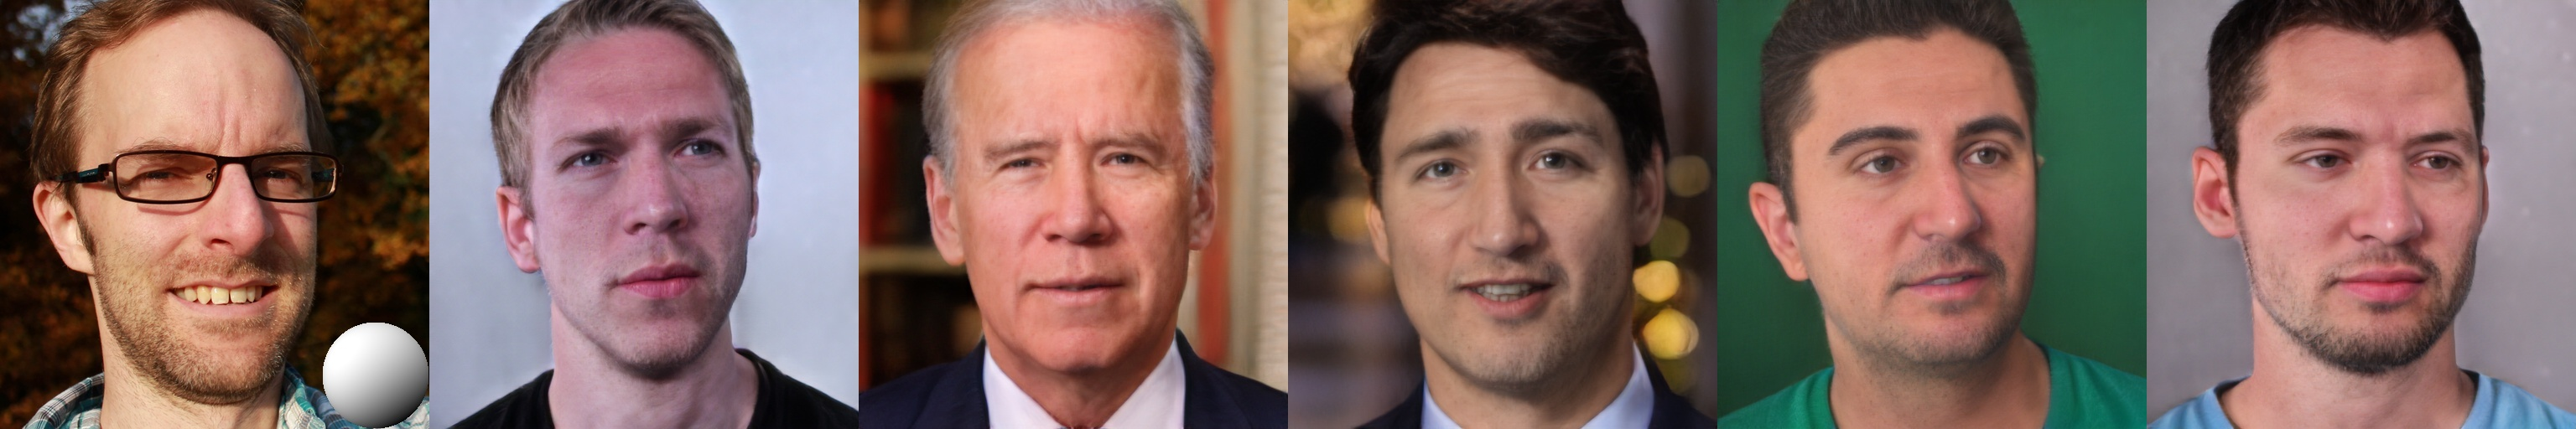}\\
\includegraphics[width=\lw]{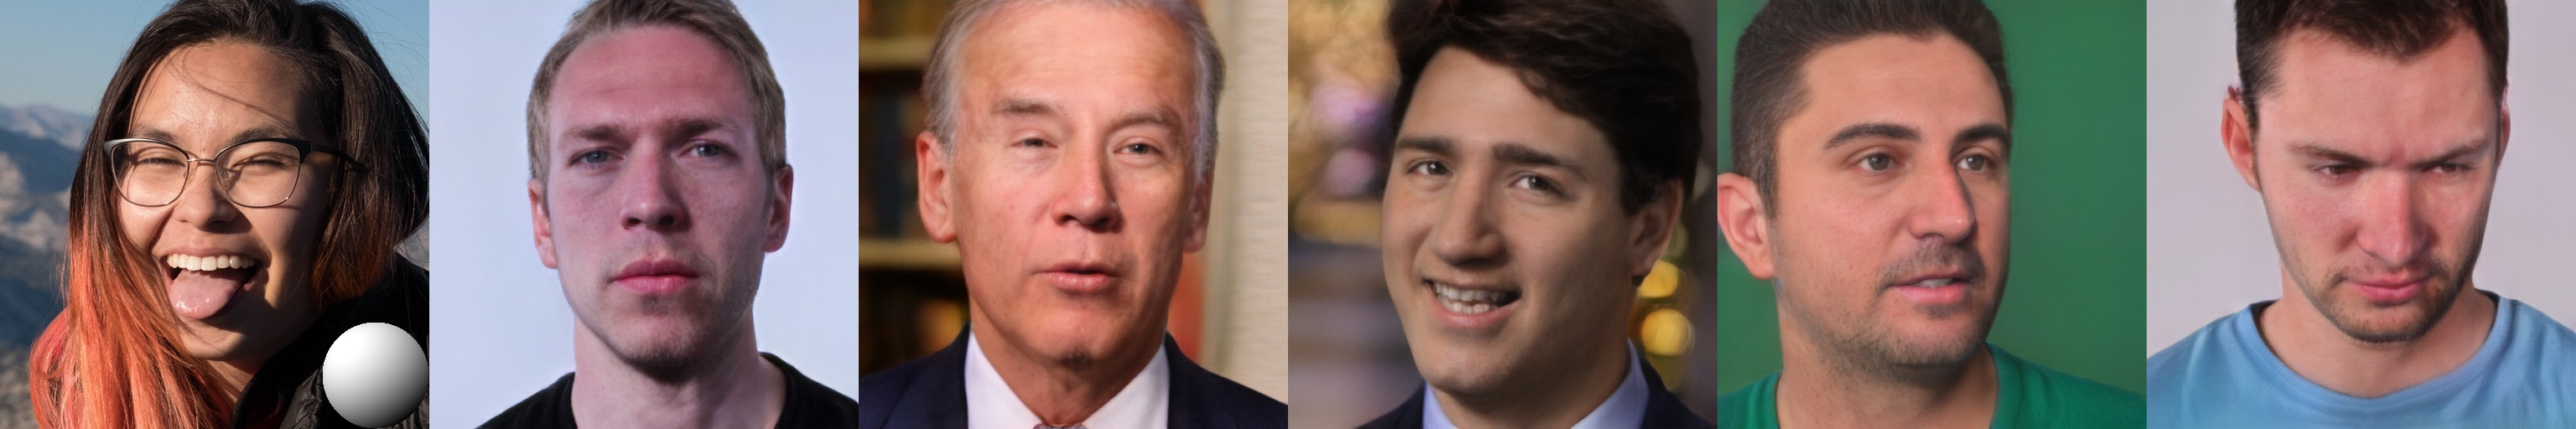}\\
\includegraphics[width=\lw]{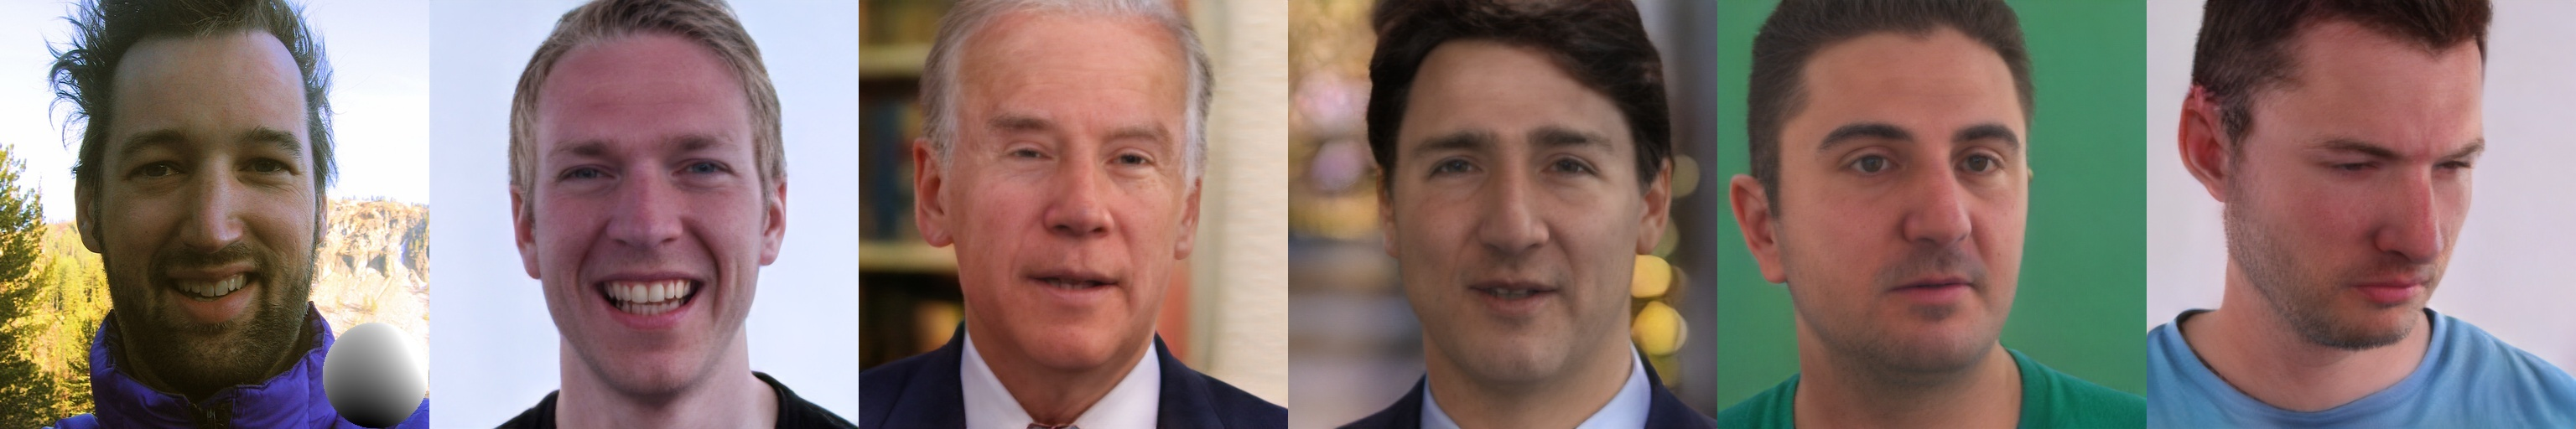}\\
\includegraphics[width=\lw]{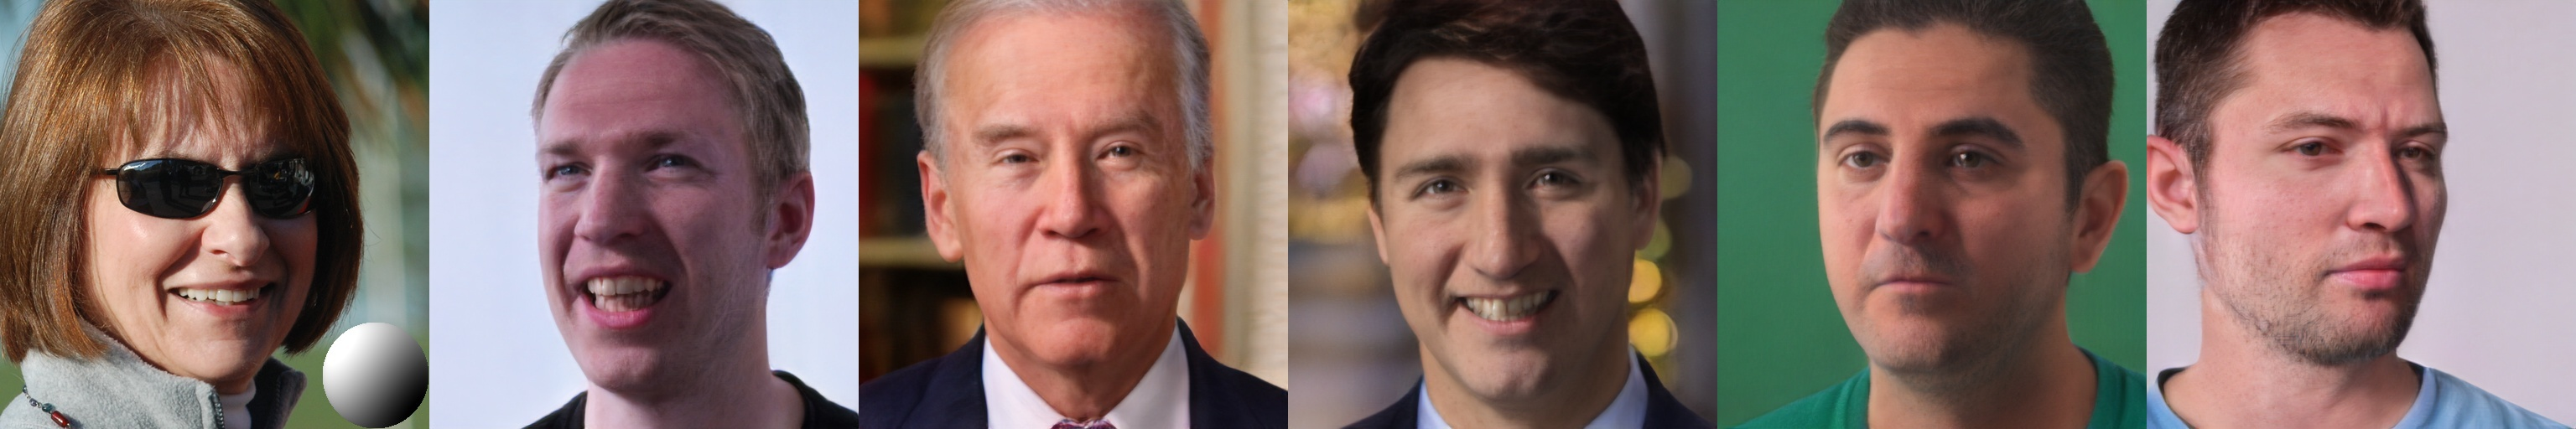}\\
\includegraphics[width=\lw]{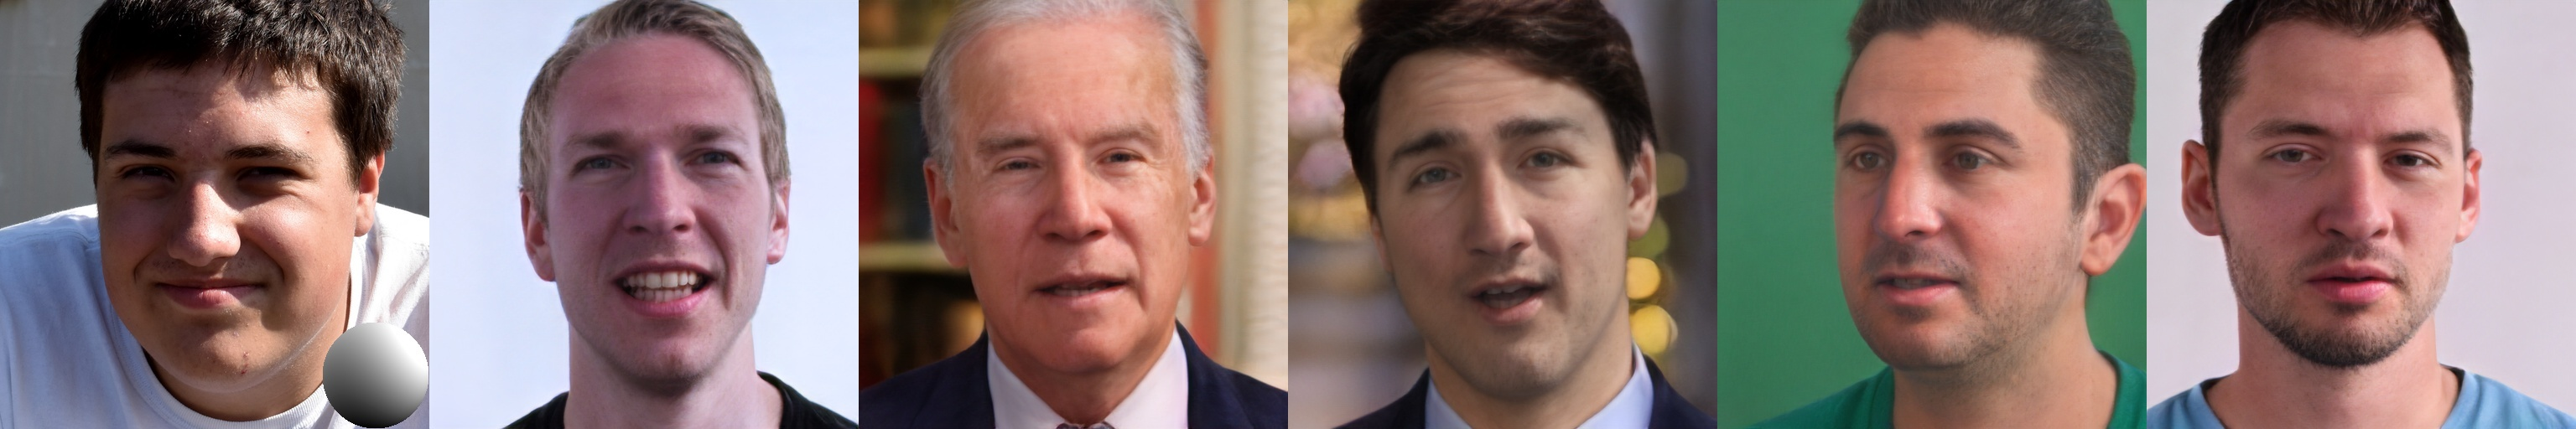}\\
\includegraphics[width=\lw]{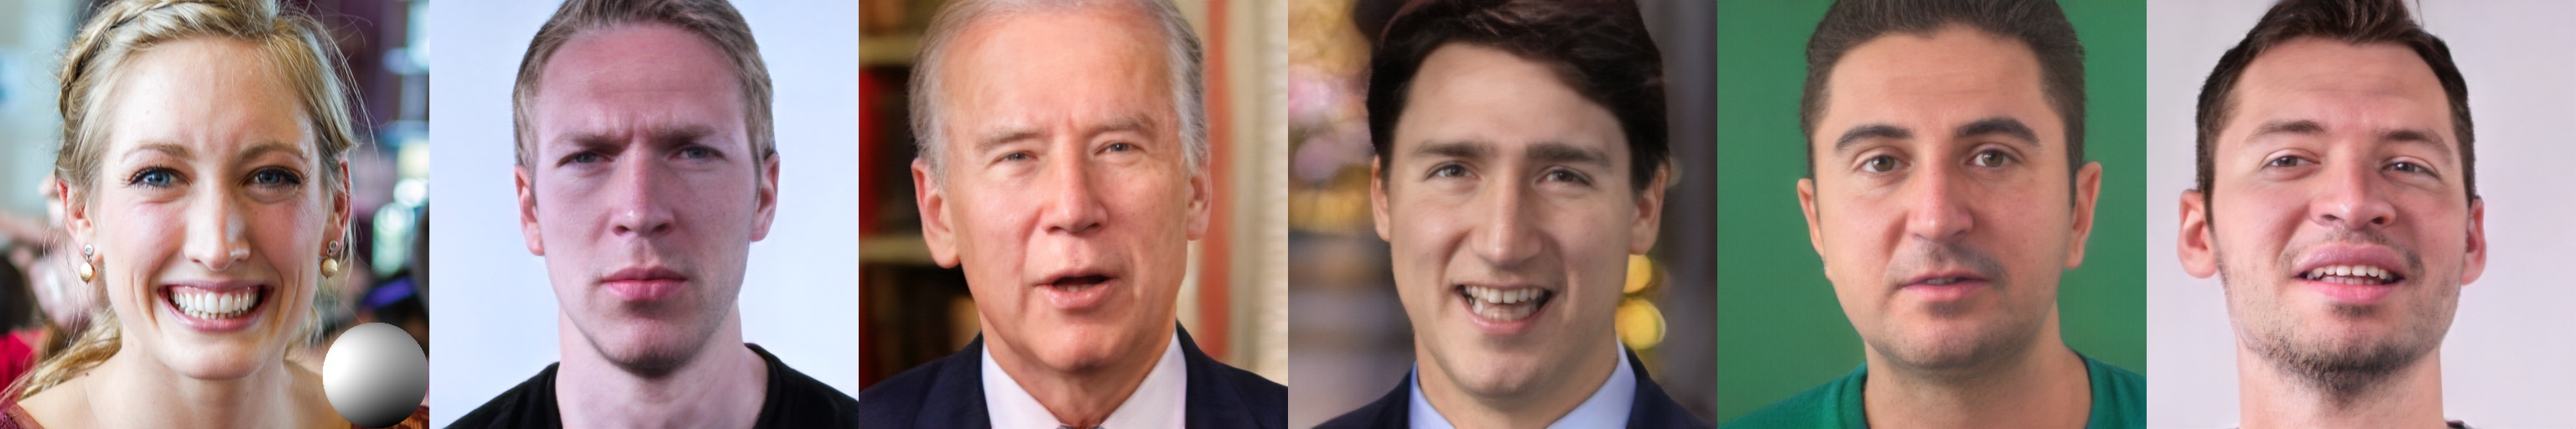}\\
\end{tabular}
\caption{Additional %
qualitative results obtained by applying our relighting technique to an input video through a lighting transfer task. The reference image is displayed in the leftmost %
column, serving as a visual anchor, while the subsequent columns exhibit the corresponding frames under distinct lighting conditions. }
\label{fig:additional novel view relighting}
\end{figure*}

\section{Implementation Details}

\paragraph{Shading Encoder.} The shading encoder appends three layers of Convolutional Neural Network (CNN) with LeakyReLU activation on top of two StyleGAN2 blocks, enabling the synthesis of shading tri-planes directly conditioned on both an albedo tri-plane and a specified lighting condition.

\paragraph{Temporal Consistency Network.}
The proposed Temporal Consistency Network leverages a combination of self-attention within a branch and cross-attention across two branches to enhance temporal consistency in processing tri-plane sequences. The network is specifically designed to operate on $n$ pairs of albedo tri-planes and shading tri-planes, where we empirically set $n$ to be 5 for optimal performance. The architecture of the Temporal Consistency Network comprises four 8-headed transformers with 4 layers, with each transformer block having a hidden size of 512. To introduce non-linearities and enhance the expressive power of the network, additional CNN blocks with ReLU activation are placed before and after the transformer-based processing. These CNN blocks employ a kernel size of $1\times 1$.

\paragraph{Superresolution Module.}
We augment the superresolution module~\cite{chan2022efficient} by incorporating an extra convolutional neural network (CNN) conditioned on a predicted albedo tri-plane. In contrast to approaches such as \cite{LP3D}, we refrain from fine-tuning the backbone model. This strategic choice not only saves time but also mitigates the risk of potential model degradation during the fine-tuning process.

\paragraph{Data Preprocessing.}
For calculating camera pose, we employ the method proposed by Deng \etal~\cite{deng2019deep3drecon}. We implement an exponential smoothing technique on the detected five facial landmarks to mitigate errors introduced during the keypoint detection process. This smoothing is applied before image cropping and camera pose calculation.

\paragraph{Data Augmentation.}
In training the tri-plane dual-encoders, we employ camera augmentation techniques similar to those outlined in \cite{LP3D}. To train the temporal consistency network, we randomly select two camera poses and perform interpolation between them to simulate consecutive frames.

\paragraph{Training.} In the initial training stage, we adopt settings from \cite{LP3D}, exclusively activating the albedo branch. This means that the model learns the intertwined representation within the albedo tri-planes. In the subsequent %
stage, we follow a fine-tuning approach inspired by \cite{nerffacelighting}. Here, we activate the shading branch to distill shading information from the entangled albedo tri-planes. This refinement ensures that the albedo tri-planes exclusively contain albedo information while the shading tri-plane encoder acquires valuable insights into shading decomposition. To train the albedo encoder, we freeze the shading tri-plane and replace the predicted shading tri-planes with the corresponding ground truth. After 32K training iterations, we freeze the albedo tri-plane encoder, substituting the predicted albedo with ground truth to exclusively train the shading encoder for an additional 32K iterations. In the final stage, we jointly train the albedo and shading tri-planes for 1.5M iterations. Furthermore, we unfreeze the albedo and shading decoders, along with the super-resolution module, with the intention of improving image quality in the overall system. After the model converges, we freeze the dual-encoder and train the temporal consistency network for 32K iterations. This multi-stage training process allows for a nuanced and comprehensive refinement of the model's capabilities.

\paragraph{Inference.}
We leverage the benefits of mixed precision and torch.compile across all network components during inference, excluding the patch embedding layer of the Vision Transformer (ViT), tri-plane decoders, and volume rendering. We sample 96 depth points per ray following EG3D~\cite{chan2022efficient}. Our model exhibits efficient resource utilization, consuming less than 4GB of GPU memory.

\begin{figure}
    \centering
    \includegraphics[width=1\linewidth]{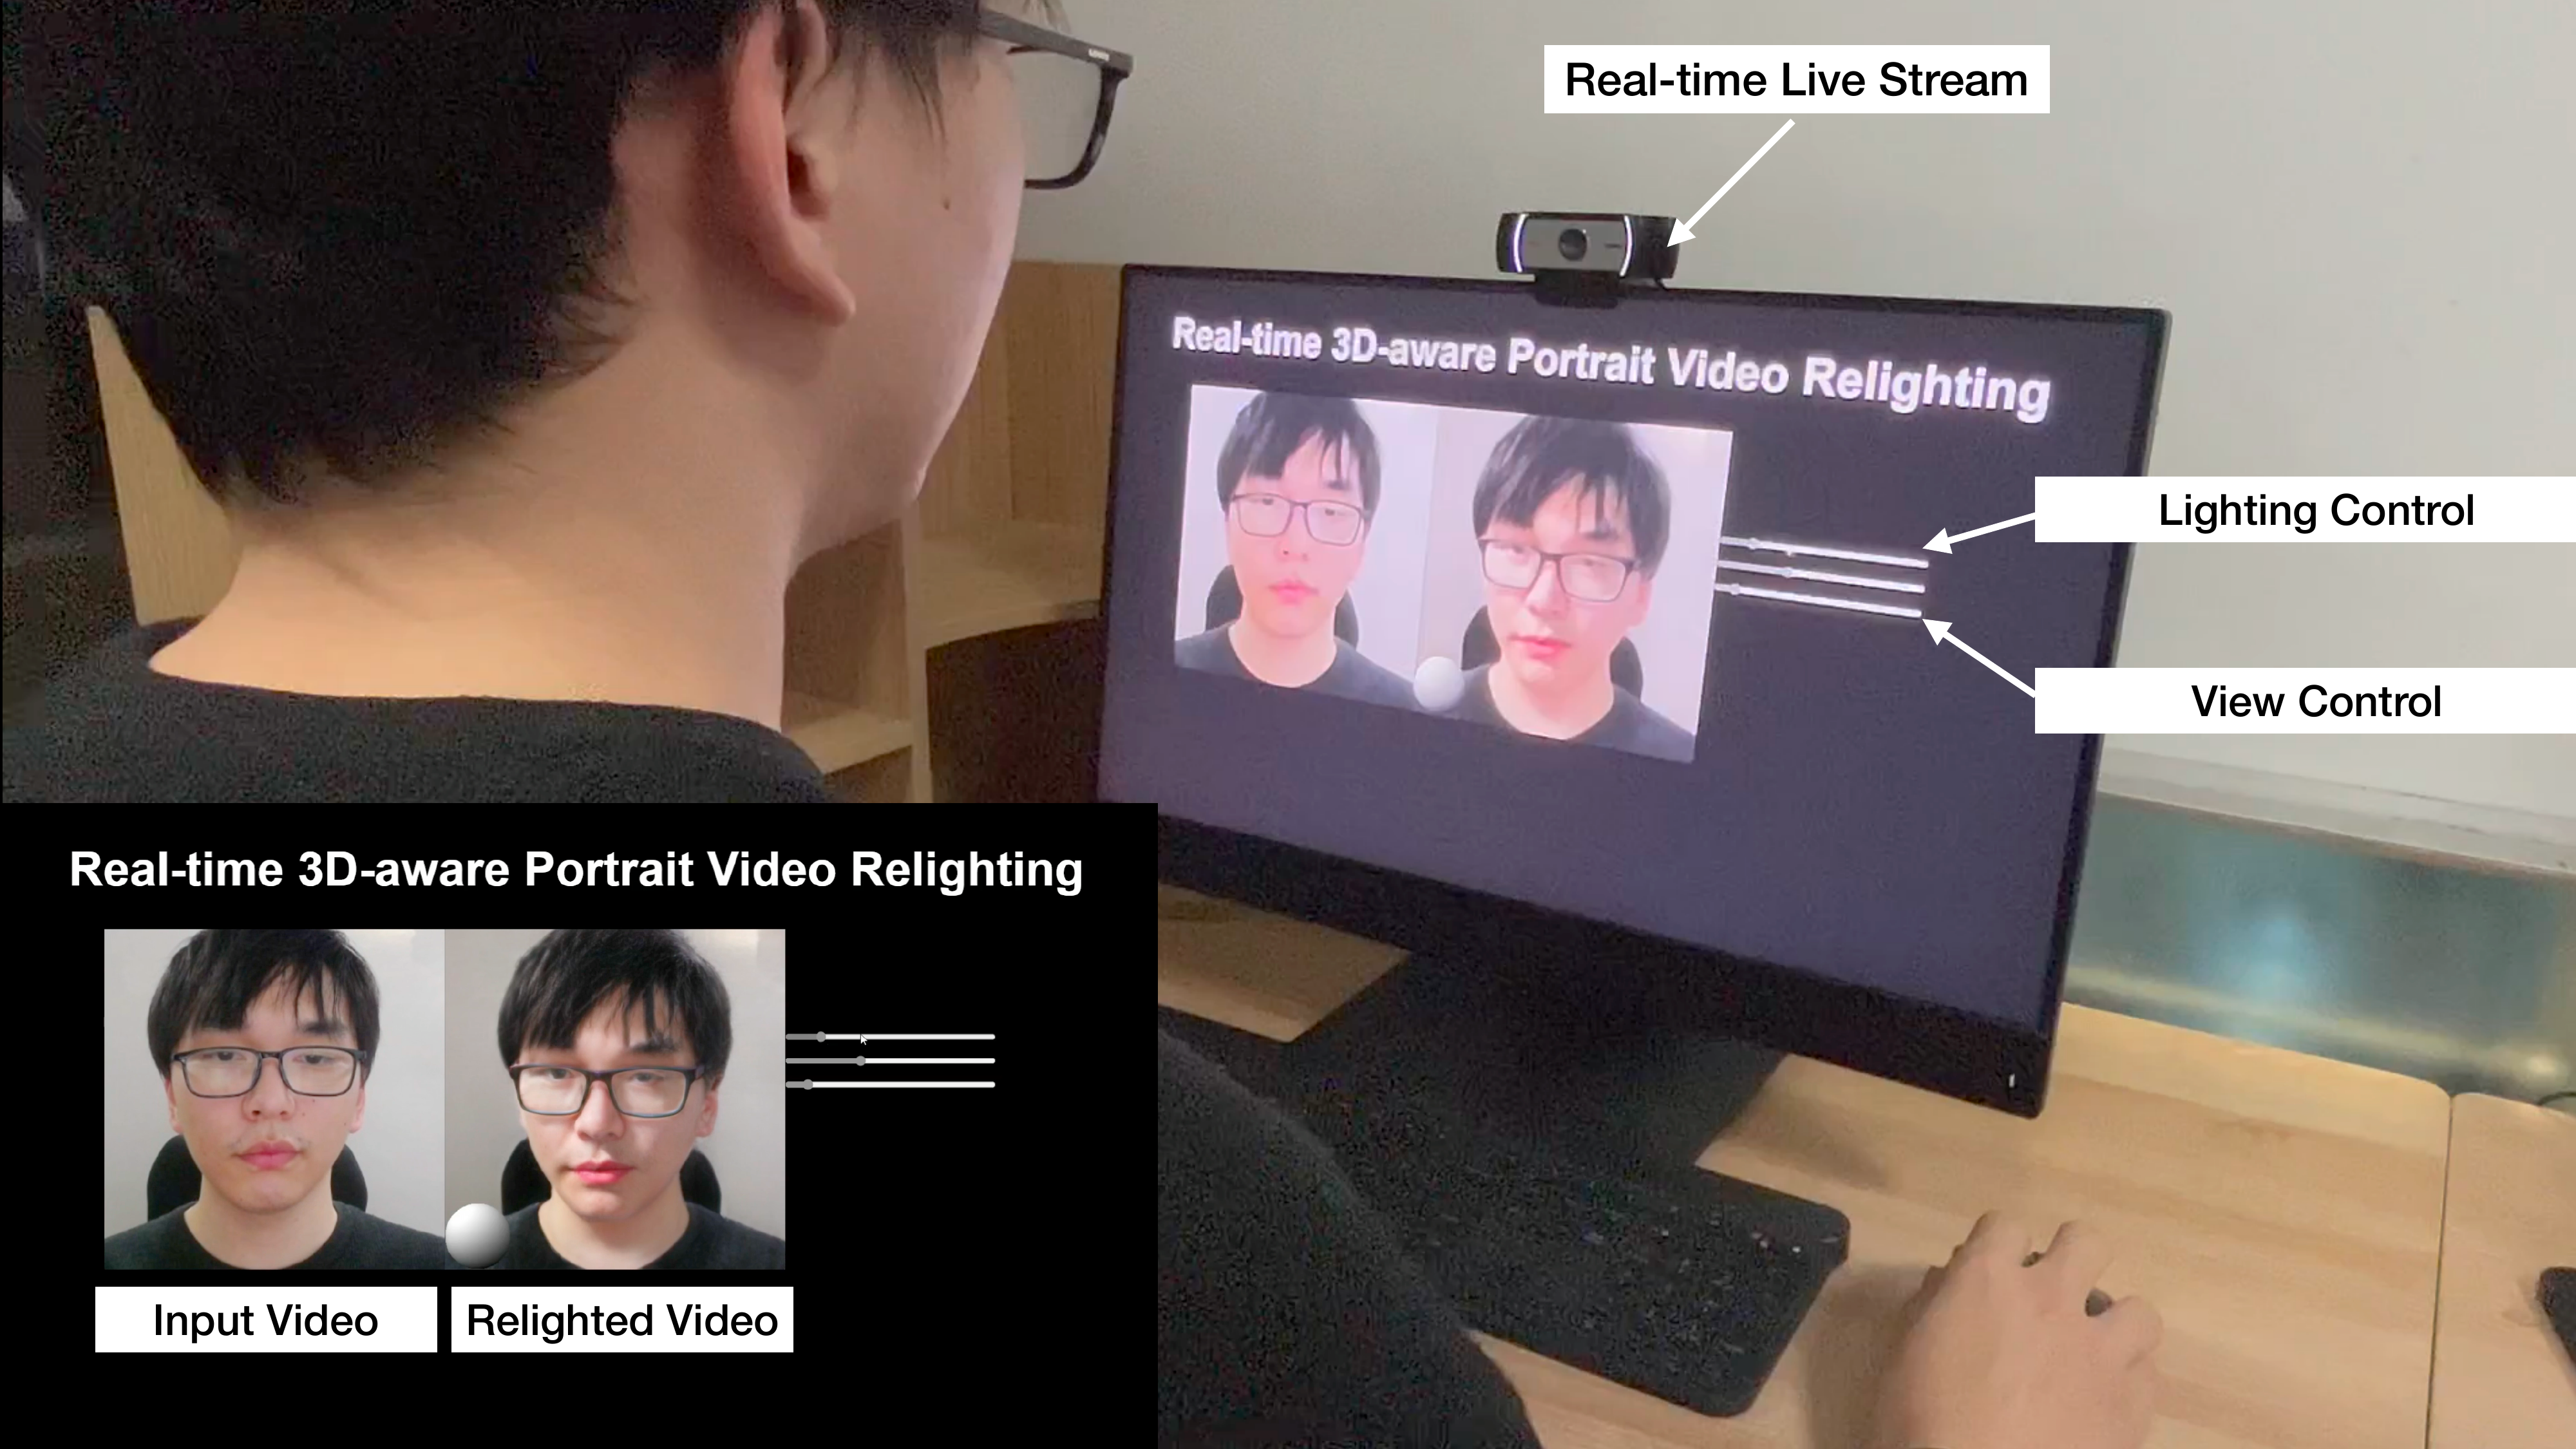}
    \caption{Our method is able to lift in-the-wild live stream to relightable 3D faces. 
    Captured portrait at each frame is reconstructed, and rendered under a novel view and with a custom lighting condition for demonstration. 
    }
    \label{fig:system}
\end{figure}

\section{Evaluation Details}

\subsection{Baselines}

For all the baselines, we use official codes and pre-trained checkpoints.

To construct our baselines using PTI~\cite{roich2022pivotal}, we modify %
the official code release (https://github.com/danielroich/PTI) %
to suit EG3D. We optimize one generator for each video clip, which involves iterating over the latent code in $\mathcal{W}+$ space of each frame for 500 iterations, followed by fine-tuning the generator for a duration equivalent to 10 times the number of frames. For PTI on NeRFFaceLighting, we use the official code release and a pre-trained encoder model (https://github.com/IGLICT/NeRFFaceLighting), which initiates the optimization process using the output latent code in $\mathcal{W}$ space from the pre-trained encoder as a starting point. The latent code is optimized for 500 iterations, and the generator is fine-tuned for another 500 iterations. Furthermore, the spherical harmonic coefficients are optimized for an additional 100 iterations.

For DPR~\cite{DPR}, we use the official code release and a pre-trained model (https://github.com/zhhoper/DPR).

For SMFR~\cite{SMFR}, we use the official code release and a pre-trained model (https://github.com/andrewhou1/Shadow-Mask-Face-Relighting).

For ReliTalk~\cite{qiu2023relitalk}, we use the official code release (https://github.com/arthur-qiu/ReliTalk) to preprocess the dataset and subsequently conduct training. To ensure consistency, we tailor the training epochs according to the video length, aligning them with the example provided by the author, \ie, more epochs for shorter videos. This meticulous adjustment results in an identical number of training iterations.

For comparison with SIPR-W~\cite{wang2020single}, TR~\cite{pandey2021total}, NVPR~\cite{Zhang_2021_ICCV}, and Lumos~\cite{yeh2022learning}, we apply our method to the input provided by the authors of Lumos and then compare our output images with those respectively provided by the authors of SIPR-W, TR, NVPR, and Lumos. 
The comparison is also demonstrated in the accompanying video for clear evaluation. 
We observe a misalignment in the provided environment maps due to different coordinate conventions. To address this, we rotate environment maps by 90 degrees (counter-clockwise when viewed from the positive Z-axis) for alignment. However, a slight misalignment persists, as our coordinate system is constructed on the front of the human face, whereas others use a world coordinate system. To rectify this, we further adjust the environment map by considering the yaw angle of the human face, ensuring correct lighting direction alignment. Additionally, we re-normalize the extracted spherical harmonic (SH) coefficients to maintain consistency across comparisons. To ensure alignment, we recrop their outputs and utilize the background masking technique from \cite{MODNet} on our results.

\section{Discussion}

\paragraph{Ethical Considerations.}

While our method provides innovative capabilities in manipulating the viewpoint and lighting conditions of a portrait video clip, it is essential to acknowledge the potential for misuse. To counteract this, using advanced image analysis tools, like fake image detectors and image watermarking, can help detect and prevent deceptive practices.

\section{Application}

\paragraph{Live-stream Video Relighting System}

As shown in \Fref{fig:system}, we introduce a real-time system to lift live-stream video into relightable 3D faces. 
Users are allowed to freely adjust the camera parameters and lighting conditions. 
A live demonstration is recorded and shown in the accompanying video. 
We run our system on two NVIDIA GeForce RTX 3090 GPUs, and achieve 20 fps for rendering one view due to the preprocessing and transmission overhead. 
This performance ensures that users can seamlessly and interactively relight and render their faces under novel views.
